# Supplementary material for: Frustration and thermalisation in an artificial magnetic quasicrystal
Source: arXiv:1703.04792 ancillary file (2017-10-06)
Supplement: Supplementary file 1 [file penrose_ice_supp.pdf]

# Frustration and thermalisation in an artificial magnetic quasicrystal
Supplementary Information

Dong Shi, Zoe Budrikis, Aaron Stein, Sophie A. Morley,
Peter D. Olmsted, Gavin Burnell, & Christopher H. Marrows

July 27, 2017

In this document, we provide additional detail on seven topics: (i) how we generated the Penrose tiling pattern; (ii) how we went about the physical realisation of that pattern; (iii) how we derived the proposed low energy configuration of that pattern, including its separation into skeleton and flippable parts and the way topologically induced emergent frustration arises in it; (iv) how we carried out Monte Carlo simulations to study the effects of long-ranged interactions; (v) how its thermalised states compare to the results of Monte Carlo simulations; (vi) what that maximum level of disorder is in the skeleton of our pattern; and (vii) how we simulated the potential for thermally induced dynamics in the flippable regions of the pattern.

## S.1 Generating the Penrose tiling pattern

When first introduced by Penrose himself[1], the creation of Penrose tilings had to be done using local tile-matching rules. The first global way of deriving a Penrose tiling, the "cut and project" method, was introduced by de Bruijn[2,3], and then subsequently developed by several others[4–7]. We used this idea to generate the P3 Penrose pattern that defines the geometry of our artificial quasicrystal.

### S.1.1 Projections from hyper-dimensional lattices

Consider an $N$-dimensional cubic lattice $\Lambda$ with orthogonal unit lattice vectors $\hat{\Lambda}_i$ in an $N$-dimensional space $R$. This space can be decomposed into two subspaces: $R_{\|}$ (parallel space) and its complementary space $R_{\perp}$ (perpendicular space), of dimension $N_{\|}$ and $N_{\perp}$, respectively. A similar decomposition then occurs when projecting $\Lambda$ into these two spaces, yielding $\Lambda_{\|}$ and $\Lambda_{\perp}$, respectively. The basis vectors of $\Lambda_{\|,\perp}$ and $\Lambda$ are linked by the following transformations:

$$\hat{e}_{\|}(j) = \sum_{i=1}^{N} q_{\|_{ij}} \cdot \hat{\Lambda}_i, \tag{S1a}$$

$$\hat{e}_{\perp}(j) = \sum_{i=1}^{N} q_{\perp_{ij}} \cdot \hat{\Lambda}_i, \tag{S1b}$$

where $q_{ij}$ is a transformation matrix element, and $\hat{e}_{\|,\perp}(j)$ is a basis vector of $\Lambda_{\|,\perp}$.

Let $C$ be a unit hypercube of $\Lambda$. When it is projected into perpendicular space $R_{\perp}$, the object that is derived is called $C_{\perp}$, the size of which defines the "window". The subset of $\Lambda$ that lies with the part of $R$ that is within the window of $R_{\|}$ is called $X$: the remaining points are "cut". The points that remain uncut are projected into the space $R_{\|}$. If the

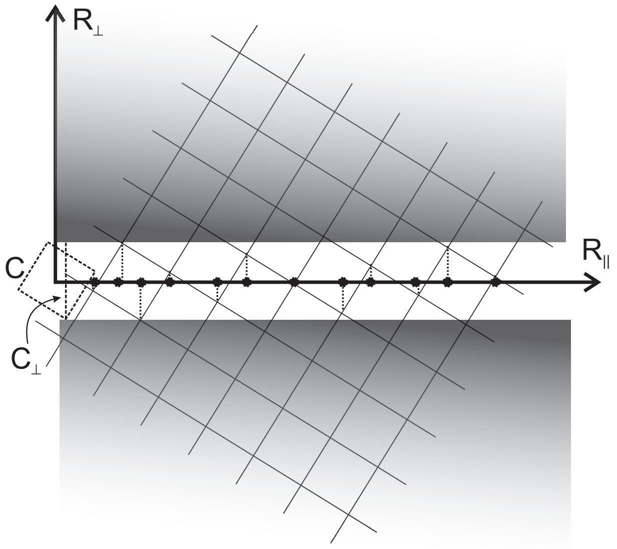


**Figure S1** | **2-D→1-D projection method.** A 2-D square lattice is aligned at an irrational slope with respect to the horizontal line (the $R_{||}$ parallel space). The square unit cell $C$ and its projection in the perpendicular space $R_\perp$, $C_\perp$ are also shown. The clear area about the horizontal line represents the section of the $R_\perp$ that lies within $C_\perp$, and each lattice vertex in this region is projected onto the horizontal line $R_{||}$ to form the 1-D Fibonacci chain.

transformation elements $q_{ij}$ are irrational numbers, then these projected points $X_{||}$ will form a quasiperiodic pattern in $R_{||}$.

### S.1.2 The Fibonacci chain: a 1-D quasiperiodic pattern

We will illustrate this with a one-dimensional example, the Fibonacci chain, which is a 1-D quasiperiodic structure. It can be generated from a 2-D square lattice, as illustrated in Fig. S1. The lattice is placed at an angle with an irrational slope with respect to the horizontal line. The slope is given by $\cos\alpha/\sin\alpha = \tau$, where $\tau = 1.618...$ is the golden ratio and $\alpha$ is the angle between the square lattice rows and the horizontal line which represents the parallel space $R_{||}$. The perpendicular space, $R_\perp$, is formed from the vertical axis in the figure. The unit cell $C$ is the rotated square that forms the lattice and $C_\perp$ is the vertical line formed by projecting $C$ on the vertical axis. All lattice points that lie within $C_\perp/2$ of the horizontal axis – in the unshaded region in the figure – are then projected onto the horizontal axis ($R_{||}$) to form the set of points comprising a quasiperiodic Fibonacci chain.

### S.1.3 The Penrose tiling: a 2-D quasiperiodic pattern

The points $X_{||}$ that form the vertices of a Penrose tiling can be obtained by projecting a 5-D hypercubic lattice into 2-D parallel subspace that has a normal parallel to the hypercube's body diagonal [11111]. In this case, the parallel space $R_{||}$ has two dimensions and the perpendicular space $R_\perp$ has three dimensions. The transformation matrices that link the bases of the lattices these subspaces and the basis of the 5-D hypercube lattice are

$$q_{||} = \sqrt{2/5}\begin{pmatrix} 1 & \cos\theta & \cos 2\theta & \cos 2\theta & \cos\theta \\ 0 & \sin\theta & \sin 2\theta & -\sin 2\theta & -\sin\theta \end{pmatrix} \tag{S2a}$$

$$q_\perp = \sqrt{2/5}\begin{pmatrix} 1 & \cos 2\theta & \cos\theta & \cos\theta & \cos\theta \\ 0 & \sin 2\theta & -\sin\theta & \sin\theta & -\sin 2\theta \\ \frac{1}{\sqrt{2}} & \frac{1}{\sqrt{2}} & \frac{1}{\sqrt{2}} & \frac{1}{\sqrt{2}} & \frac{1}{\sqrt{2}} \end{pmatrix} \tag{S2b}$$

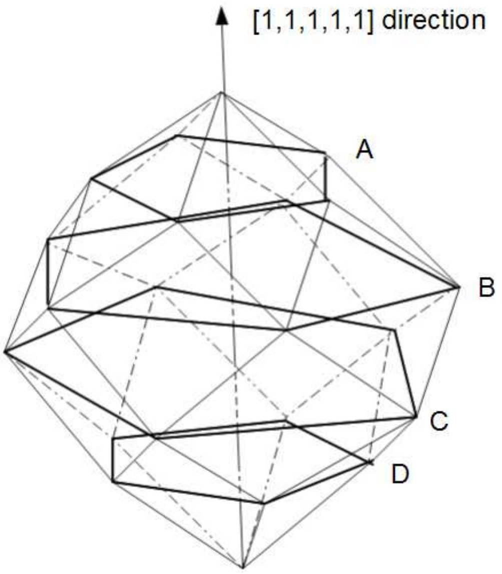


**Figure S2** | **Icosahedral space.** When a unit hypercube in 5-D is projected into a 3-D perpendicular space, a rhombic icosahedron will be formed. The points which are projected from the 5-D lattice are constrained to lie in four pentagonal planes, to which the [11111] direction forms a normal. They are marked A, B, C, and D, respectively.

where $\theta = 2\pi/5$. $C_\perp$ can, in this case, be obtained by projecting the hypercube unit $C$ into the perpendicular space $R_\perp$. It is a rhombic icosahedron, which is depicted in Fig. S2. From the matrix expression for $q_\perp$, we can see that when the points are projected onto $R_\perp$ they will sit on four planes, which are normal to the [11111] direction in the hypercubic lattice.

When a set of points $X$ within the window in the 5-D hypercubic lattice are projected into the parallel space $R_\|$, we get a set of points $X_\|$. The pattern obtained possesses tenfold rotational symmetry, and hence still is not a Penrose tiling pattern. In order to break the two-fold symmetry, another parameter $\gamma$ is introduced, which is used to shift the four planes in $C_\perp$ along the [11111] direction. It has been shown that when $\gamma$ varies from 0 to 0.5, it will generate different structures[8]. When $5\gamma = 0$ (mod 1), the pattern contains local ten-fold symmetric vertices (and is known as an anti-Penrose pattern). When $5\gamma = 0.5$ (mod 1), the structure is a Penrose tiling, which possesses a single point of five-fold rotational symmetry. Examples of these two possibilities are depicted in Fig. S3. The characteristic five-fold rotational symmetry of the penrose tiling arises from projection of the five dimensional hypercube along its body diagonal. The individual rhombi in the Penrose tilings shown in 3 are the projections of the square 2-D faces of the hypercube.

For the pattern used in the experiments reported here, the scale of the 5-D hypercube is chosen to be 3 unit lengths along each axis, and $\gamma$ is selected to have the value of 0.3. When decorated with magnetic nanoislands along its bonds, the Penrose tiling shown in Fig. S3 becomes the artificial Penrose ice depicted in Fig. 1 of the main text. This is the so-called "P3" Penrose tiling, where each tile is either a thin or a thick rhombus. All the intervertex distances are the same in this pattern, meaing that they can all be decorated with a single design of nanoisland.

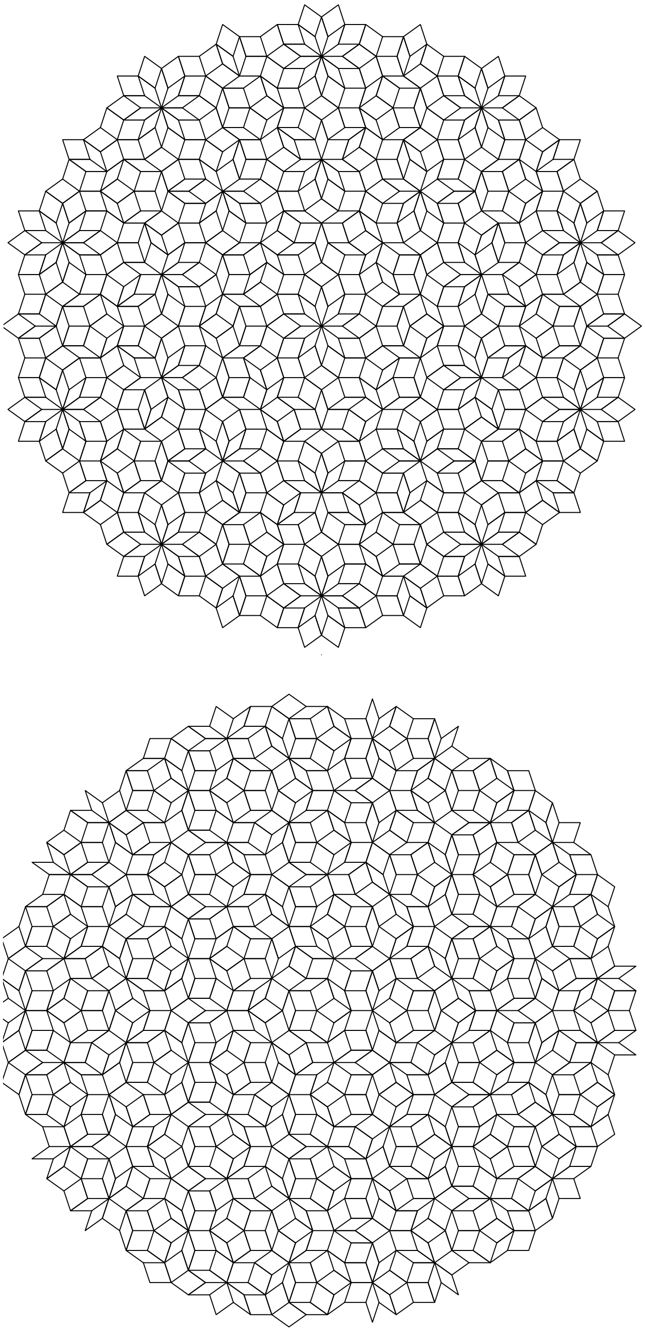

**Figure S3 | Tilings generated by different values of $\gamma$.** Top: When choosing $\gamma = 0$, the pattern contains ten-fold rotationally symmetric vertices and is an anti-Penrose pattern. Bottom: When choosing $\gamma = 0.3$, the pattern is the fivefold rotationally symmetric P3 Penrose tiling that is studied in this work.

# S.2 Design and fabrication of the artificial quasicrystal pattern

Having defined our P3 tiling pattern, we now turn to the arrangement of macrospins upon it. Vedemdenko *et al.* considered XY spins on the vertices of a P3 pattern[9]. As Bhat *et al.*[10] and Farmer *et al.*[11] did with their P2T patterns, we choose Ising-like macrospins on the bonds of the array. However, we have not connected them so that the coupling strength may be varied by moving them closer together or further apart. We therefore designed magnetic nanoislands that would exhibit single domain Ising-like macrospin behaviour and that are compatible with the P3 tiling geometry.

The drawing of the different vertex types in Fig. S6 shows that in many of the them, the magnetic nanoislands meet at acute angles. This means that the nanoislands must have sharply pointed tips in order to be able to be brought close enough together to be able to reach the strongly coupled regime. We therefore designed the shuttle-shaped nanoisland that is shown in Fig. S4, which we used in all of our experiments. Both experiment and simulation show that it reliable forms a single domain state to provide the Ising-like macrospin needed in this work.

In Fig. S5 we show scanning electron micrographs of examples of the artificial magnetic quasicrystal arrays with intervertex spacing 600 nm and 1000 nm. The close-up view of the 600 nm array in panel Fig. S5a shows the need for the sharply pointed tips on the shuttle-shaped nanoislands. It is important to note that in the P3 tiling, all the bonds are the same length and so all the islands are nominally identical. This means that will all have nominally the same blocking temperature, which is proportional to island volume. This is important in our thermal annealing experiments, where all islands can thermalise on a equal basis. If we had used a P2T kite-and-dart pattern, for instance, with two different tile edge lengths, we would have had two groups of islands that froze at different temperatures during cooling.

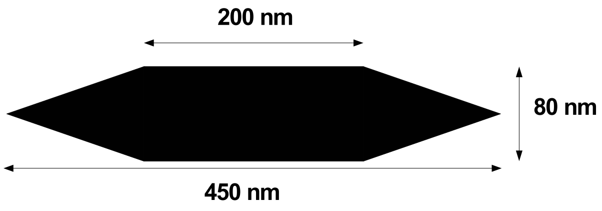


**Figure S4 | Shuttle-shaped nanoisland design.** The sharp points allow the nanoislands to meet at the acute angles found in vertex types IV, VI, and VII.

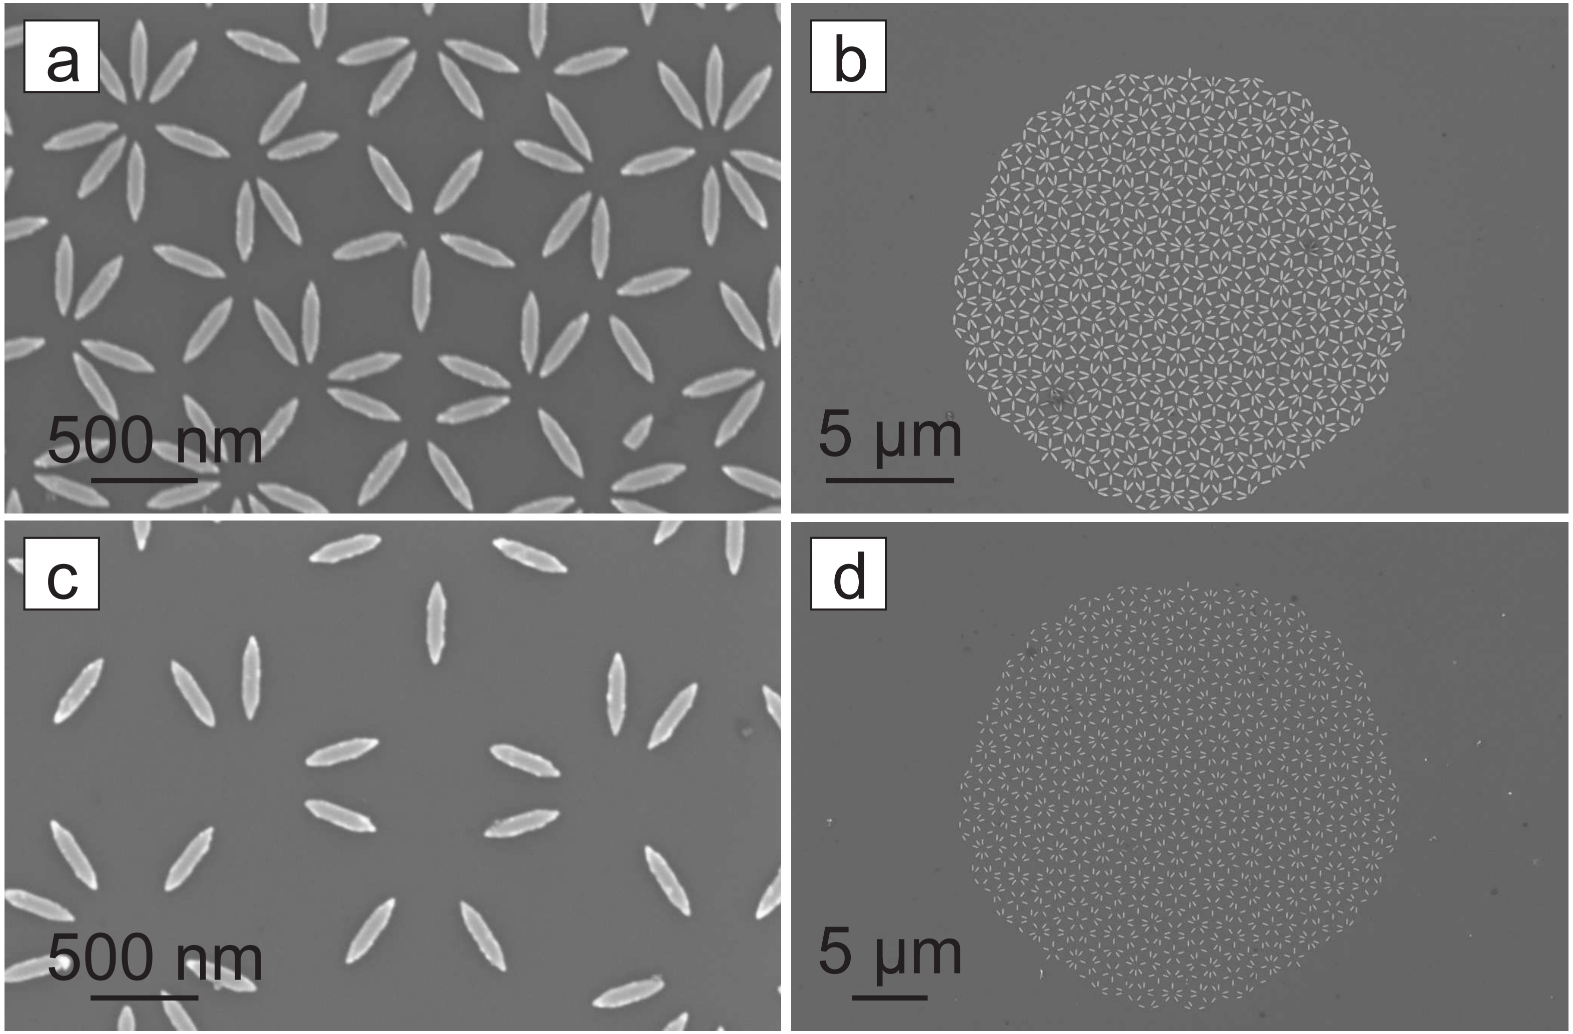


**Figure S5** | **Scanning electron micrographs of artificial magnetic quasicrystals. a**, Close-up view and **b**, overview of a 600 nm intervertex spacing array. **c**, Close-up view and **d**, overview of a 1000 nm intervertex spacing array.

## S.3 Low energy configurations of the P3 Penrose artificial magnetic quasicrystal

Having defined the nature of the array (a P3 Penrose tiling) and of the spins that decorate it (Ising-like spins on its bonds), we now turn in this section to the questions of how the energies of this system were calculated and thus how a state of global lowest energy may be constructed. We adopt a step-by-step logical process, joining islands into vertices, vertices into decagons, and decagons into the completed pattern, determining the lowest energy configurations at each point. It reveals the two emergent features discussed in the main text: the separation of the pattern into an ordered skeleton and flippable clusters (previously observed as the outcome of more opaque Monte Carlo simulations [9,11]), and presence of topologically induced emergent frustration (previously seen in the periodic shakti lattice [12]). The step-by-step process allows insights into how these emergent features arise in the context of quasiperiodic artificial spin systems.

### S.3.1 Single-vertex low energy states

The Penrose tiling pattern that we have studied possesses seven different vertex geometries, as shown in Fig. 1 of the main text and Fig. S6 in this document. The energies of the lowest and next lowest energy configurations for each vertex have been calculated based on micromagnetic simulations of isolated vertices with realistic island shapes carried out using the OOMMF software package [13]. We used the standard parameters for Permalloy, given in the methods section. Since our islands are disconnected, the only interactions between them are magnetostatic in nature, with minor modifications to the vertex energies due to canting of spins at the island tips away from a perfectly uniform state. The pointed shapes of the tips means that these modifications are very small.

The results, along with the calculated energy gaps between the ground state and first excited state of each vertex, are shown in Fig. S6, with the gaps normalised to the smallest value, that for a type VII vertex. For certain cases–the ground states of the type I and type V vertices and the first excited states of the type II and type VII vertices–there is already a single spin that is degenerate, and hence "flippable", due to vertex-level frustration. It is worth noting that this means that as the vertices are excited, the degeneracies are affected.

### S.3.2 Tiling the vertices to form the Penrose spin ice

When these vertices are tiled together to form the Penrose spin ice, it can be verified by inspection that the ground state vertices cannot be joined together compatibly. Thus, *topologically induced emergent frustration* is present. This means that in order to find a ground state of entire system, we need to maximise the occurrence of the lowest energy configurations for as many vertices as possible, whilst minimising the number (and thus the energy cost) of excited vertices that are compatible with the global configuration. Due to the lack of spatial periodicity, the brute-force method of finding the low energy configuration is to tile the Penrose pattern vertex-by-vertex, searching for these incompatibilities at each step, which is a rather tedious process.

On the other hand, the Penrose pattern can be decomposed into overlapping decagons, which are projections of the 5D hypercubic unit cell. In our scheme there are two different decagon units–which we denote A and B–each of which contain several vertices. Examples of each of which are shown in Fig. S7. This suggests a more efficient strategy, the details of which are given below. As a first step, the low energy configuration of each of the decagons will be determined, and then the ground state of the entire pattern will be constructed based on joining these decagons into a low energy configuration. It is important to note that whilst our decagon-based scheme of construction shares some similarities with that of Gummelt, described in reference 14, it is not exactly the same. We use smaller decagons with different overlaps, and also have to consider magnetic properties, not just structural ones.

| Vertex type | I | II | III | IV | V | VI | VII |
|---|---|---|---|---|---|---|---|
| Ground state | 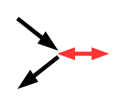 | 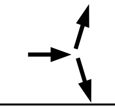 | 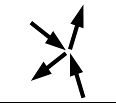 | 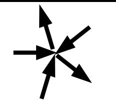 | 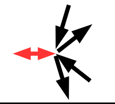 | 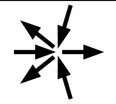 | 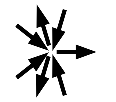 |
| First excited state | 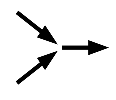 | 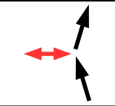 | 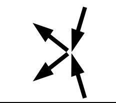 | 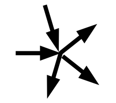 | 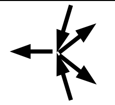 | 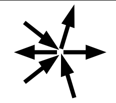 | 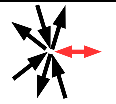 |
| Energy difference | 9.141 | 1.885 | 9.141 | 18.27 | 3.477 | 15.93 | 1.00 |

**Figure S6 | Low energy configurations of the seven types of vertex.** The lowest and next lowest magnetic configurations of each vertex type are shown. In each case the states are twofold degenerate, in that a configuration in which all the moments are flipped will have the same energy. The red double-headed arrows represent moments that possess their own degeneracy: the direction of this moment may be reversed without affect the the total energy of vertex. The energy difference between level one and two has been normalised by that of type VII vertex. The energy calculations were performed using the OOMMF micromagnetic simulation package.

#### S.3.2.1 Lowest energy configuration of the type A decagon

The type A decagon has a two-fold mirror symmetry in its vertex structure. The lowest energy configurations of the vertices found in the decagon turn out to all be compatible with each other. The construction process of the lowest energy state is shown in Fig. S8. The global configuration in decagon A can be easily inferred from a single element orientation: this figure shows an example where the magnetic moment orientation of a single element is chosen, and vertex-by-vertex, the entire decagon is populated with macrospins. The vertex-level degeneracy of one macrospin remains–marked in red in Fig. S8–but that of two others is lifted by joining into the decagon pattern. The outermost ring of ten macrospins may form a flux-closed ring circulating in either direction at this stage (and so is not marked in the diagram) but, since these macrospins will be shared with overlapping decagons when the complete covering of the Penrose tiling is formed, their eventual direction will be constrained by these overlaps.

#### S.3.2.2 Lowest energy configuration of the type B decagon

The type B decagon has a fivefold rotational symmetry, and so, as shown by the dashed lines in Fig. S9, it can be divided into five equal parts. We consider just one of these to begin with. At the centre of this part is a type II vertex. Examining the entire pattern, we can see that the vertex at the edge of the decagon (the next nearest neighbour) may be of type III or type I.

Taking the case of type III first, then it is not possible for both vertices to be in their vertex-level lowest energy states, as is shown in Fig. S9a(i) and a(ii), unless the nearest neighbour (type V) vertex is excited out of its lowest energy state, as shown in Fig. S9a(iii), which has a much higher energy cost according to Fig. S6 and is thus very unlikely. The excited vertex is drawn in red in each case. Topologically induced emergent frustration has arisen.

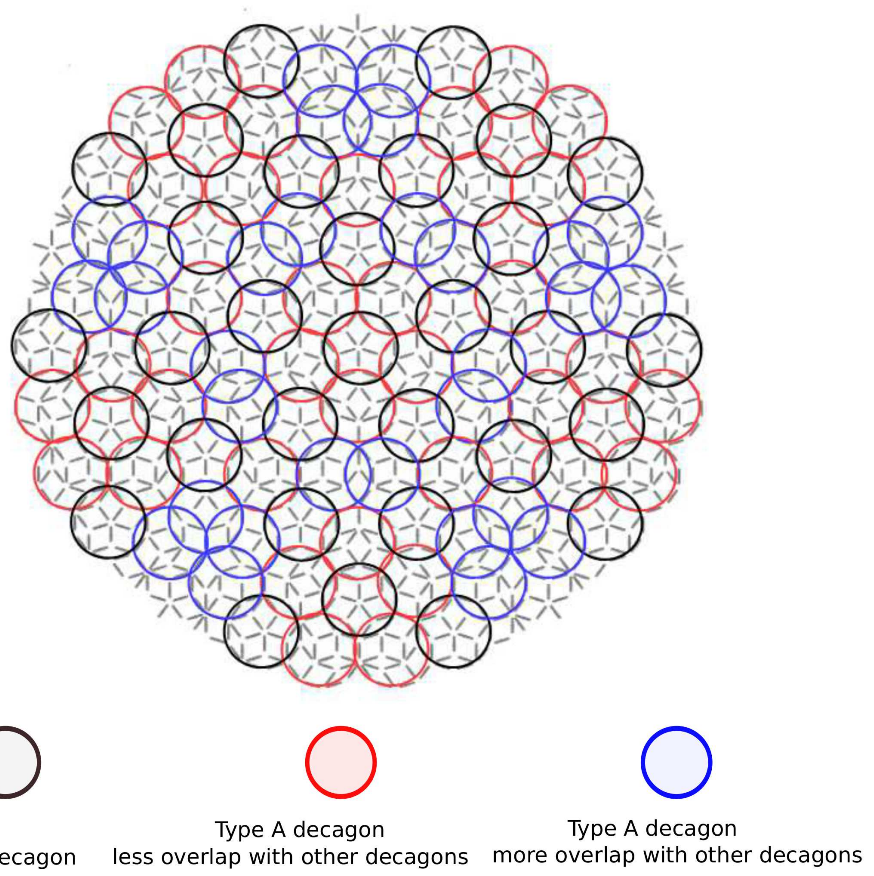


**Figure S7 | The decagon units in the P3 Penrose tiling pattern.** The P3 Penrose tiling can be decomposed into two types of overlapping decagons, highlighted here by circles of different colour. The type A decagons have a mirror symmetry and are highlighted by red or blue circles, depending on the nature of their overlaps with their neighbours. Type B decagons have a fivefold rotational symmetry and are marked with black circles. Only three situations arise where decagons overlap, as explained in more detail below in Fig. S10. An overlap of a red/blue and a black decagon corresponds to cases (a) and (c) in that figure, in which overlaps are limited to a single thin rhombus. The larger three-rhombus overlaps between two blue decagons correspond to case (b).

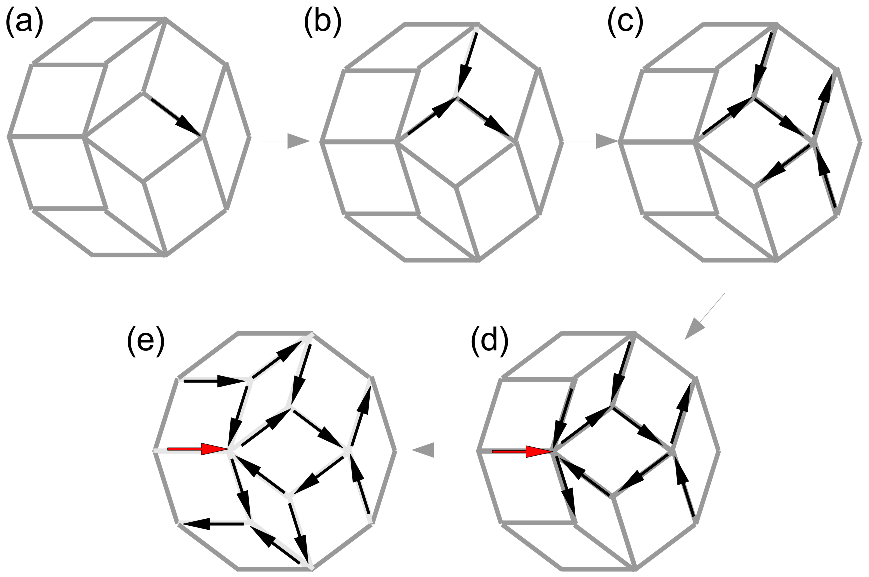


**Figure S8** | **Type A decagon ground state construction process.** **a**, by assuming a single element magnetic moment direction is given, **b**, then the favourable magnetic moment directions of the neighbour islands can be inferred from configurations in Fig. S6. **c**, and **d**, more islands magnetic configurations can be inferred from the lowest energy configurations in Fig. S6. The red arrow denotes the sole moment that can point in either of the two directions without costing extra energy. **e**, the moment direction of the remaining islands inside the decagon can be worked out following similar rules: two vertex level degeneracies are lifted when they join the decagon pattern.

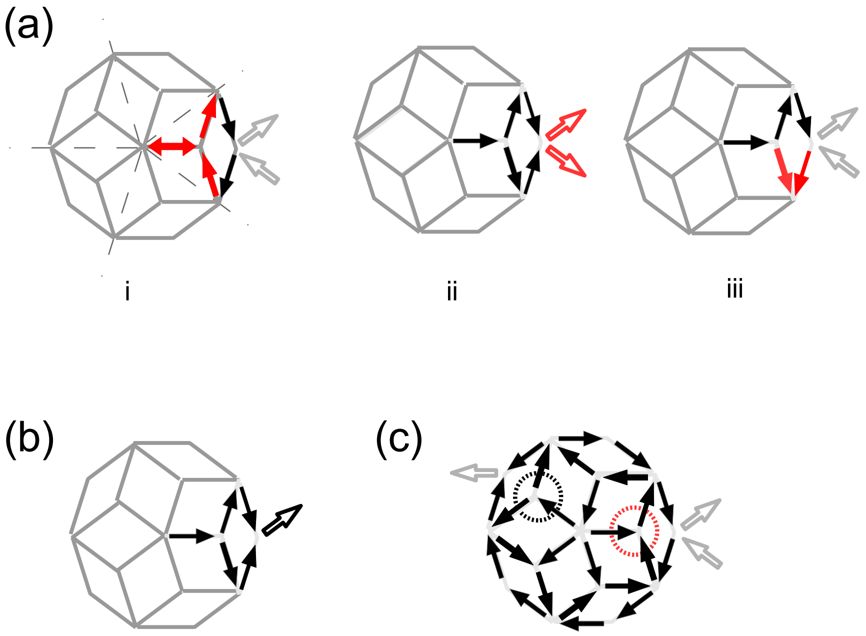


**Figure S9** | **Type B decagon ground state construction.** **a**, a type B decagon can be divided into five equal parts, as indicated by the dashed lines. Each part has a type II vertex at its centre. If the edge (next nearest neighbour) vertex is of type III, then one of them cannot be in the lowest energy configuration, as shown in diagrams **a**i and **a**ii. The only way to avoid this is to pay the very high energy cost of putting an intermediate (nearest neighbour) vertex into a higher energy configuration (**a**iii). In these three diagrams, the vertex lifted out of its lowest energy state is drawn in red, and the open arrows represent the macrospins that are not formally part of this decagon. **b**, if the edge vertex is of type I, then both it and the central type II may stay in their lowest energy configurations. **c**, a low energy configuration of a type B decagon. Two type II vertices are in different energy levels (as denoted by the black and red circles) due to their different environments.

On the other hand, if the edge vertex is a type I vertex, then both of these vertices can remain in their lowest energy state, as shown in Fig. S9b. In this case, the remaining vertices in the decagon can all take up their lowest energy state after proper tiling.

Hence, the exact lowest energy configuration of a type B decagon depends on the neighbouring islands in its immediate environment (see Fig. S9c). Certain type II vertices must be excited through topologically induced emergent frustration.

#### S.3.2.3 Joining the decagons

When overlapping the decagons to construct the full Penrose pattern, three particular cases need special consideration.

1. When a type A decagon overlaps with one of type B, both decagons can stay in their lowest energy states, as shown in Fig. S10a. The type IV vertex at the centre of the type B decagon, which is drawn in red, may remain in its lowest energy configuration, but has ten different possible ways to do this. It thus forms a ‘flippable’ cluster of macrospins, surrounded by the rigid ‘skeleton’.

2. When a mirrored pair of type A decagons are overlapped, two of the type II vertices

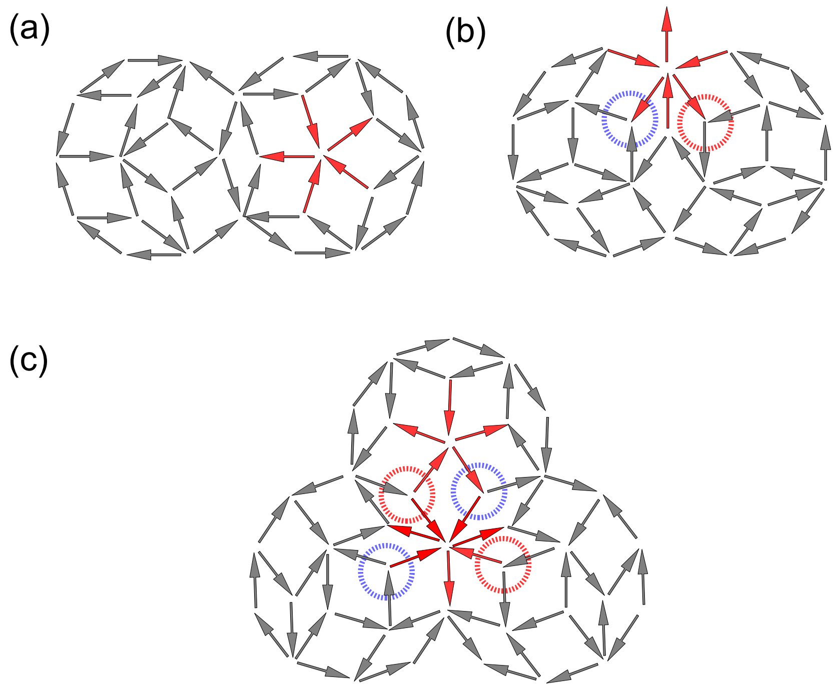


**Figure S10** | **Three cases of connected decagons.** **a**, a type A and a type B decagon are joined together. Both decagons can stay in the lowest energy state in a compatible manner. The red arrows represent the macrospins at a type IV that has a high degree of degeneracy: it is flippable and may take up any variant of the lowest energy configuration without altering the overall energy. **b**, when two type A decagons are joined together, there are two type II vertex that cannot both be in their vertex-level lowest energy states simultaneously, which are represented by the blue and red circles. One of these two vertices has to be lifted to its first excited state level (red circle), which results in an intermediate type VI vertex (red arrows) being forced into one of its two degenerate states. **c**, two type A decagons joined with one of type B. The four type II vertices are not compatible with each other (red and blue circles), which leads to two of them lifting their energy level to the first excited state (red circles). As a result, a type VII and a type IV vertex, drawn using red arrows, are each forced into one of their two degenerate states.

are not compatible with each other, as shown in Fig. S10b). The frustration may be overcome by lifting either one of them to a higher energy level, which will force an intermediate type VI vertex, drawn using red arrows, to take up one of its two degenerate states. This will be switched into the other state if the two frustrated vertices interchange their configurations, which costs no energy. This is another example of how topologically induced emergent frustration can arise.

3. When two type A decagons are joined with one of type B decagon, as shown in Fig. S10c, there will be four type II vertices that experience topologically induced emergent frustration. This results in two of them being lifted into higher energy levels, which will force each of an intermediate type VII and a type IV vertex, drawn in red arrows, into a particular one of their two degenerate states. These again may be switched if the energy levels of the four frustrated type II vertices are interchanged, at zero total energy cost.

### S.3.3 The lowest energy configuration of the whole pattern

Taking all of the above into consideration, the lowest energy configuration of the whole pattern can be tiled decagon by decagon. The final construction is shown in Fig. S11. The rigid skeleton is shown in black in one form of its long-range ordered ground state. The other form is straightforwardly obtained by inverting every black macrospin.

The red and blue arrows represent the macrospins that are flippable and collectively lead to macroscopic degeneracy of the entire pattern. Consequently, the system has a large residual entropy. The total number of degenerate states is $W = 2 \times 2^{70} \times 10^{46}$, where 70 and 46 are the numbers of vertices in the flippable part with degeneracies of 2 and 10, respectively. This implies a ground state entropy $S = k_B \ln W \simeq 155 k_B$. The entropy density then can be estimated as $S/(N_{\mathrm{spins}} k_B) = 0.094$ for the $N_{\mathrm{spins}} = 1650$ P3 macrospin system. This can be compared with the entropy per macrospin found in the kagomé ices: $S/(N_{\mathrm{spins}} k_B) = 0.501$ (Ice I) and $S/(N_{\mathrm{spins}} k_B) = 0.104$ (Ice II) [15]. Note that we have converted the results reported by Zhang *et al.* from information entropy (in logarithm base 2) to thermodynamic entropy (natural logarithm).

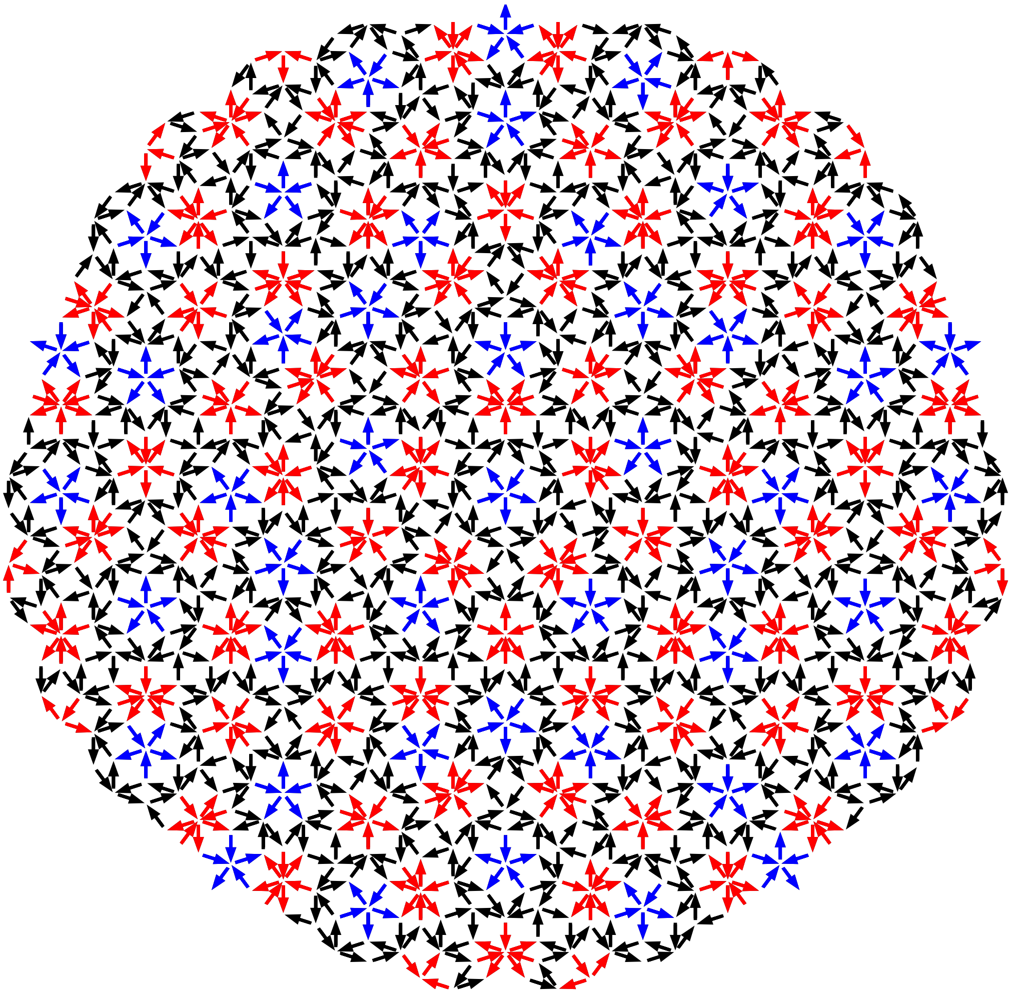

**Figure S11 | The lowest energy configuration of the whole Penrose spin quasicrystal.** The pattern consists of 1,650 macrospins that separate into two parts. The skeleton part (black arrows) consists of type I, II, III, and IV vertices, and has a unique long-range ordered ground state. The flippable part (red arrows and blue arrows) consists of clusters of type V, VI, and VII vertices. The different colours, red or blue, are used to illustrate the clusters of macrospins, with degeneracies of 2 and 10, respectively. Each of these clusters can take up one of its degenerate configurations without changing the total energy of the pattern, leading to macroscopic degeneracy for the pattern as a whole.

## S.4 Monte Carlo simulations of long range interactions between flippable clusters

Under the approximation of nearest-neighbour interactions between islands used in §S.3, the ground states of the system are exactly extensively degenerate due to the presence of the flippable clusters. However, in finite-sized systems with long-range interactions this degeneracy becomes a *quasidegeneracy*, due to dipolar interactions favouring ordering of flippable spins to, e.g., flux-closed loops where possible. In addition, boundary conditions play a role and the average environment of spins near the system edges is different from those near the centre. We therefore hypothesise that degeneracy lifting is at least partly governed by finite size effects, and as the system size increases the energy difference between states with fixed skeleton spins but differing flippable spins should become small.

To investigate the effect of long-range interactions, we studied states energetically close to the ground state by performing short Monte Carlo simulations, as described in the methods section, at low temperature on a system with a proposed ground state as its initial configuration. (The proposed ground state is exactly one of the ground states of the system when interactions are short-ranged only.) As in our other Monte Carlo simulations, each island was replaced by an Ising spin placed at its centre, with anisotropy parallel to the long axis of island, and spins interacted by dipole-dipole interactions with all other spins in the system. We studied systems of size $N_{\mathrm{spins}} = 770$, 1,650, and 3,150 spins, and performed 20,000 independent simulations of each system size. Each starts from the same proposed ground state, but the probabilistic nature of the Monte Carlo method means that many different final states are reached.

In Fig. S12a, we show the density of energy states $\mathcal{N}(e_{\mathrm{dip}}/e_0)$ attained in short simulations (up to $\sim 20$ accepted spin flips per simulation) for the 1650-spin system with inverse temperature $\beta = 1$. We rescaled the average dipole-dipole energy per spin of the entire pattern $e_{\mathrm{dip}}$ by a characteristic per-spin energy difference $e_0$, which is defined as the difference in energy/spin between level 1 and level 2 of an isolated type I vertex. The density $\mathcal{N} = N(e_{\mathrm{dip}}/e_0)/(\Delta e_{\mathrm{dip}}/e_0)$, where $N$ is the number of configurations obtained with energies in a bin $[e_{\mathrm{dip}}, e_{\mathrm{dip}} + \Delta e_{\mathrm{dip}})$, with bin size $\Delta e_{\mathrm{dip}}/e_0 = 2 \times 10^{-3}$. Also indicated are the energies of the initial configuration (solid vertical line) and the energies of other proposed ground state configurations of this system, that is, configurations that are energetically degenerate with the initial configuration under the approximation of short-range interactions (dashed vertical lines). The spread of energies of states found in the simulations is similar to the spread of energies of proposed ground states, indicating that the energy difference between the lowest-energy state found and the highest is small, and that the configurations generated in simulations are all quasi-degenerate ground states. The degeneracy is only split by $0.004/5.6 \approx 0.1\%$ of the ground state energy.

The effect of system size is shown in Fig. S12b, which shows how the standard deviation $\sigma$ in energies found in simulations depends on system size $N_{\mathrm{spins}}$. In order to standardize procedures for all system sizes, we run each simulation until one accepted spin flip is found, consider only unique configurations found via this method, and measure the standard deviation over the same number of randomly-chosen samples for each system size. (In practice, this is set by the number $n = 42$ of unique configurations found for the smallest system size $N_{\mathrm{spins}} = 770$.) The decrease in $\sigma$ for larger system sizes $N_{\mathrm{spins}}$ indicates that the quasi-degeneracy of ground states becomes closer to exact degeneracy in the thermodynamic limit. We conclude that the nearest-neighbour model used in this paper is therefore a useful approximation to the true energetics of the system.

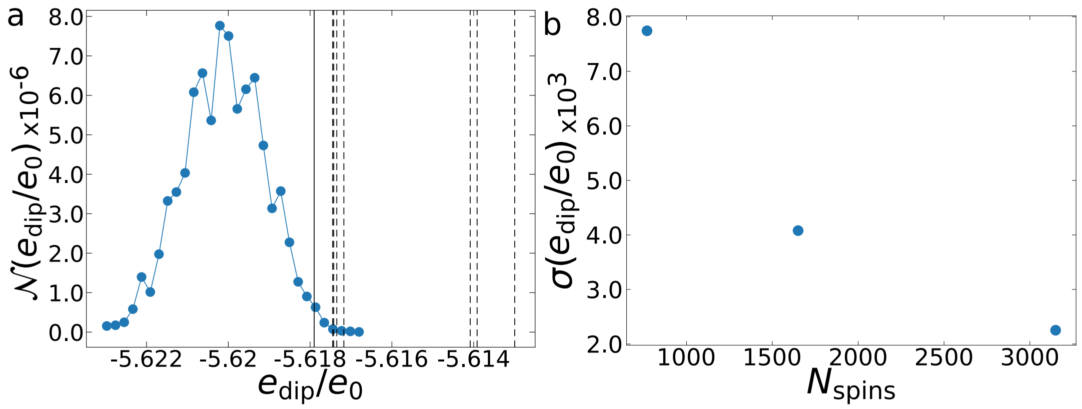


**Figure S12 | Monte Carlo simulations of low-energy states show long-range interactions lead to small energy differences between quasi-degenerate states. a**, distributions of energies of states obtained from 20,000 simulations for a $N_{\rm spins} = 1,650$ system relaxed from a proposed GS at inverse temperature $\beta = 1$. The solid vertical line is the energy of the initial configuration, the black dashed lines are the energies of typical configurations where "flippable" spins have been flipped, that is, configurations that in the approximation of short-range interactions are energetically degenerate. **b**, standard deviation of energies of configurations attained from proposed GSs via a single Monte Carlo accepted spin flip at $\beta = 1$. In both panels, the energies are scaled by system size and are given in units of a characteristic per-spin energy difference $e_0$ which is the difference in energy/spin between level 1 and level 2 of an isolated type I vertex.

## S.5 Skeleton states: experiment vs. simulation

In Fig. S13 we compare the measured populations of the energy levels in the thermally annealed and as-grown skeleton states with the results from the Monte Carlo simulations for the same quantities. The experimental data are for the 600 nm intervertex spacing array. The simulation was carried out in a strong coupling regime with $e_0/k_\mathrm{B}T = 0.8$, where $e_0$ is the difference in energy/spin between level 1 and level 2 of an isolated type I vertex. This is equivalent to the 600 nm pattern at its blocking temperature of $T_\mathrm{B} = 696$ K with a magnetisation of $M_\mathrm{s} = 72$ kA/m. The experimental value of $N_\mathrm{spins} = 1,650$ was used.

In Fig. S13a we show the data for the thermally annealed array with a line of best fit, which has slope $0.90 \pm 0.03$ and intercept $0.028 \pm 0.008$. This is close to the case of a perfect match, which would have a slope of unity and zero intercept. The data are also rather well clustered around the straight line, with an adjusted $R^2$ value of 0.97.

Meanwhile, in Fig. S13b we show the equivalent plot for the as-grown array. In this case the line of best fit has slope $0.56 \pm 0.06$ and intercept $0.06 \pm 0.02$. This falls far short of the ideal match. The data are also less well-described by a simple stright line fit, with an adjusted $R^2$ value of 0.68.

This representation of the data reinforces how closely the thermally annealed system comes to the results of the Monte Carlo simulation, and how different the as-grown magnetic configuration of the skeleton is.

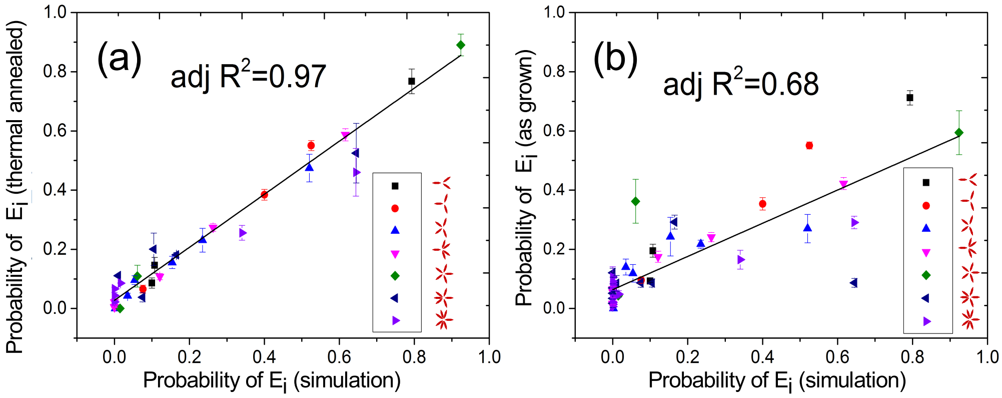


**Figure S13 | Comparison of experimental skeleton states to Monte Carlo simulations. a**, the observed occupation probability of each energy level $E_i$ of each vertex in the thermally annealed state plotted against the same probabilities as determined from the Monte Carlo simulation. **b**, the observed occupation probability of each energy level $E_i$ of each vertex in the as-grown state plotted against the same probabilities as determined from the Monte Carlo simulation. Both experimental data sets are from the average of three patterns with 600 nm lattice spacing, whilst the simulation results are from an average of ten configurations. The solid lines are lines of best fit, and the adjusted $R^2$ of each data set is given in each panel.

## S.6 Maximum number of domain walls in the P3 Penrose skeleton

It is useful to compare the level of disorder we observe in our differently prepared skeleton states to the maximum possible level.

We parameterise the level of disorder through the number of domain walls, $L$. The maximum number of domain walls in the skeleton, $L_{\mathrm{max}}$, can be calculated as follows. A reasonable definition of the system being totally disordered is that for each vertex all the energy levels are equally populated. $L$ is defined as the number of vertices in the excited states. So, when the system is totally disordered, $L_{\mathrm{max}}$ can be calculated as the total number of vertices in the excited states. This can be evaluated for each vertex type. For instance, for type I vertex, of which there are 110, in our Penrose tiling, $E_1$ has a 4-fold degeneracy, $E_2$ has a 2-fold degeneracy, and $E_3$ has a 2-fold degeneracy, as shown in Fig. 2a. Hence the probability that a given type I vertex is in an excited state is $2+2$ out of a total of $4+2+2$ which is $4/8 = 0.5$. Hence, the total number of type I vertices in excited states when system is totally disordered is expected to be $0.5 \times 110 = 55$. The other skeleton vertex types (types II, III, and IV) can be treated in similar way, except for the type II vertices. For those there is an exception, due to the effects of the topologically induced emergent frustration that we have addressed just above. In ground state of our Penrose pattern, only 105 of the type II vertices stay at $E_1$ and 190 of them have to be excited to $E_2$. For a type II vertex we have $E_1$ with 2-fold degeneracy, $E_2$ with 4-fold degeneracy, and $E_3$ with 2-fold degeneracy. We should therefore perform the calculation as $6/8 \times 105$ (number of vertices not in $E_1$) $+4/8 \times 190$ (number of vertices not in $E_2$).

Putting all this together, the maximum number for the pattern that we have studied is given by:

$$L_{\mathrm{max}} = 0.5 \times 110 + 0.75 \times 105 + 0.5 \times 190 + 0.875 \times 65 + 0.875 \times 180 = 443.$$

## S.7 Monte Carlo simulations of thermally induced dynamics

In order to study the distribution of spins that flip at finite temperature, we performed MC simulations on a 1650-spin system at various temperatures. In each simulation, we make $10^9$ attempted MC moves. Figures S14a and S14b show the spatial distributions of spin flip probabilities for inverse temperatures $\beta e_0 = 500$ and $\beta e_0 = 10$ respectively, where $e_0$ is an energy scale defined by the energy difference between level 1 and level 2 of a type I vertex. The total number of spins that flip in our simulations increases with temperature, as shown in the inset of Fig. S14c. At low temperatures ($\beta e_0 = 500$; Fig. S14a), no skeleton spins flip. As temperature is increased skeleton spins have an increased flipping probability, however even at $\beta e_0 = 10$ (Fig. S14b) the only skeleton spins that flip are located on the system boundary and have fewer near neighbours than skeleton spins in the bulk. As temperature is increased further, the flipping probability tends to become equal for all spins. This trend can be observed in the histogram of flipping probabilities (Fig. S14c), where at $\beta e_0 = 10$ there is a 'pile up' of the distribution near $P_{\mathrm{flip}} = 1/1650 \approx 6 \times 10^{-4}$.

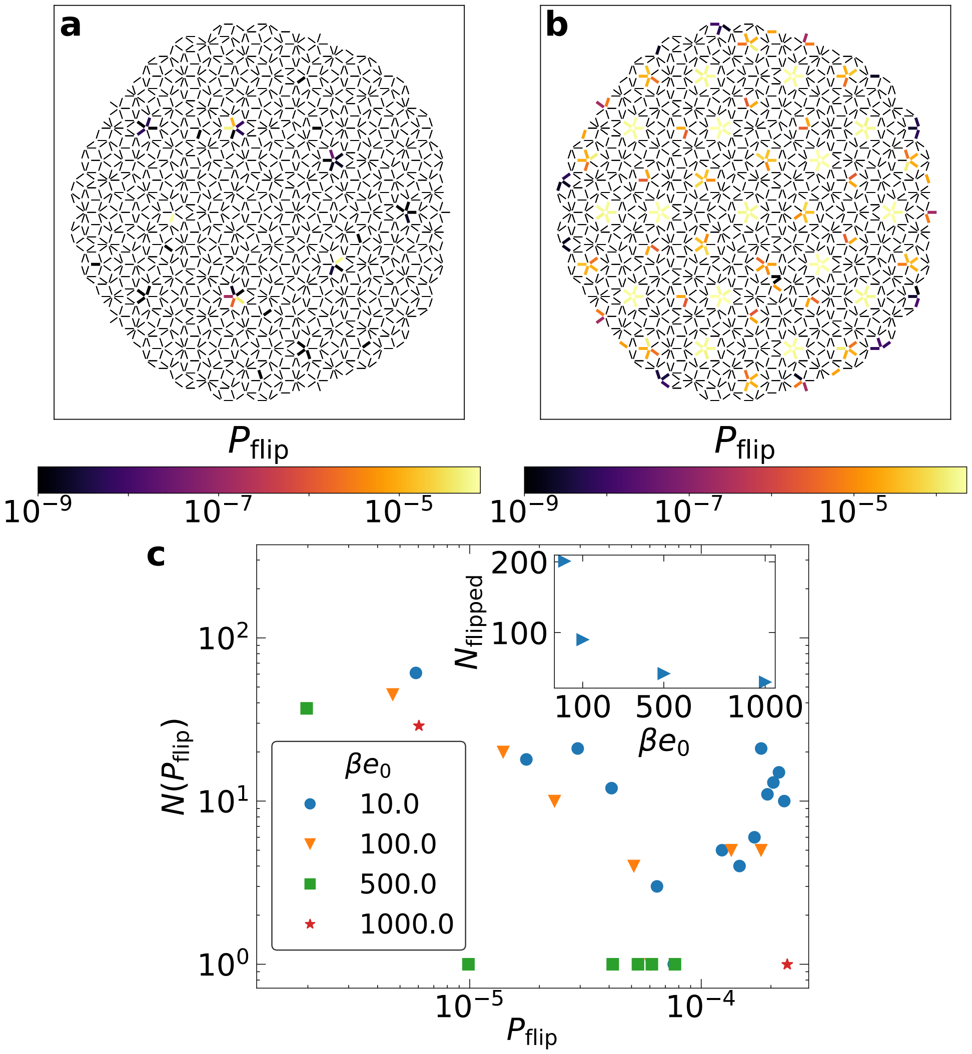


**Figure S14 | Monte Carlo simulations show how the probability of a spin flipping depends on temperature.** Spatial distributions of spin flips for inverse temperatures **a**, $\beta e_0 = 500$ and **b**, $\beta e_0 = 10$, where the energy scale $e_0$ is the energy difference between levels 1 and 2 of a type I vertex. Spins that have flipped in the course of the simulation are drawn as thick lines and coloured according their flip probability $P_{\text{flip}}$, defined as the number of flips of a spin divided by the number of attempted MC moves. Spins that have not flipped at all have $P_{\text{flip}} \ll 10^9$, and are drawn as thin black lines. **c**, Distribution of the number $N$ of spins with a given probability of flipping during a simulation, $P_{\text{flip}}$. The inset shows the number of spins that flip in a simulation as a function of inverse temperature.

# References


[1] Penrose, R. The rôle of aesthetics in pure and applied mathematical research. *Bull. Inst. Math. Appl.* **10**, 266 (1974).

[2] de Bruijn, N. G. Algebraic theory of Penrose's non-periodic tilings of the plane. I. *Indagationes Math. (Proceedings)* **84**, 39 (1981).

[3] de Bruijn, N. G. Algebraic theory of Penrose's non-periodic tilings of the plane. II. *Indagationes Math. (Proceedings)* **84**, 53 (1981).

[4] Kramer, P. & Neri, R. On periodic and non-periodic space filings of $E^m$ obtained by projection. *Acta Cryst. A* **40**, 580 (1984).

[5] Duneau, M. & Katz, A. Quasiperiodic patterns. *Phys. Rev. Lett* **54**, 2688 (1985).

[6] Elser, V. The diffraction pattern of projected structures. *Acta Cryst. A* **42**, 36 (1986).

[7] Ishihara, K. N. & Yamamoto, A. Penrose patterns and related structures. I. superstructure and generalized Penrose patterns. *Acta Cryst. A* **44**, 508 (1988).

[8] Whittaker, E. J. W. & Whittaker, R. M. Some generalized Penrose patterns from projections of $n$-dimensional lattices. *Acta Cryst. A* **44**, 105 (1988).

[9] Vedmedenko, E. Y., Oepen, H. P. & Kirschner, J. Decagonal quasiferromagnetic microstructure on the Penrose tiling. *Phys. Rev. Lett.* **90**, 137203 (2003).

[10] Bhat, V. S. *et al.* Controlled magnetic reversal in permalloy films patterned into artificial quasicrystals. *Phys. Rev. Lett.* **111**, 077201 (2013).

[11] Farmer, B. *et al.* Direct imaging of coexisting ordered and frustrated sublattices in artificial ferromagnetic quasicrystals. *Phys. Rev. B* **93**, 134428 (2016).

[12] Gilbert, I. *et al.* Emergent ice rule and magnetic charge screening from vertex frustration in artificial spin ice. *Nature Phys.* **10**, 670 (2014).

[13] Donahue, M. J. & Porter, D. G. OOMMF User's Guide, Version 1.0. *Interagency Report NISTIR 6376, National Institute of Standards and Technology, Gaithersburg, MD* (1999). URL `http://math/nist.gov/oommf`.

[14] Gummelt, P. Penrose tilings as coverings of congruent decagons. *Geometriae Dedicata* **62**, 1 (1996).

[15] Zhang, S. *et al.* Crystallites of magnetic charges in artificial spin ice. *Nature* **500**, 553 (2013).
